# Supplementary material for: Secure and Efficient Watermarking for Latent Diffusion Models in Model Distribution Scenarios
Source: arXiv:2502.13345 source file (2025-02-18)
Supplement: Supplementary file 1 [file appendice.tex]

% \begin{abstract}
% This document presents supplementary materials supporting our main submission. In section \ref{sec1} , we provide more details on parameters for watermarking method. In section \ref{sec2}, we analyze the influence of watermark capacity on the bit accuracy and image quality. In section \ref{sec3}, we analyze the impact of the sampling method. In section \ref{sec4}, we present additional evidence to establish the robustness of DistriMark. In section \ref{sec5}, we provide some information on the efficiency of watermark embedding.
% \end{abstract}

% \section{1.Parameters for Watermarking Methods}
% \label{sec1}
% \noindent \textbf{Stable Signature \cite{fernandez2023stable}, FSwatermark\cite{xiong2023flexible}} We use the pretrained watermarked variational autoencoder provided in the paper which embeds 48-bit  and 100-bit messages partially. The watermark-related parameters are consistent with the default settings of the implementation code in the paper. Images are generated using 25 inference steps.

% \noindent \textbf{Tree Ring. \cite{wen2024tree}} We evaluate the Tree-Ring$_{rings}$ method, which the authors state “delivers the best average performance while offering the model owner the flexibility of multiple different random keys”. Using the author’s implementation, we generate and verify watermarked images using 25 inference steps, where we use an empty prompt during verification and keep the remaining default parameters chosen by the authors. The evaluation standard for detection is p-value.

% \noindent \textbf{DwtDct \cite{cox2007digital}, DwtDct \cite{cox2007digital}, RivaGan \cite{zhang2019robust}.} We utilize a 48-bit watermark for DwtDct and DwtDct, and a 32-bit watermark for RivaGan. Default parameters from the Stable Diffusion implementation are maintained.

% \noindent \textbf{Parameters for DistriMark.} The watermark embedded in the robustness evaluation is 48-bit watermark. The watermarked images are generated and verified using 25 inference steps. An empty prompt is used for diffusion inversion. The version of the variational autoencoder used for fine-tuning is Stable-Diffusion-2-1-base \cite{rombach2022high}. The skip connection method is multi-level connections. The parameter settings in the attack layer are as follows: Gauss Blur with a kernel size $7\times7$ and std of 0.01, Gauss Noise(std.) in [0.1,0.8], Brightness in [0.5,1.5], Contrast in [0.5,1.5] and JPEG in [50,90].  The balancing weight $\varepsilon=0.8$, $\delta=0.05$.

% \section{2.Analysis on Watermark Capacity.}
% \label{sec2}
% %对于水印容量，实验分别嵌入了16、32、48、64、96比特水印以探究DistriMark水印容量对于图像质量的影响。
% For embedding capacity, the experiment embedded 16, 32, 48 and 64 bits of DistriMark watermark to investigate its influence on image quality. The main results are shown in Table \ref{tab1:capacity}. When the watermark capacity is within 48 bits, there is no significant difference in image quality parameters such as NIQE, PIQE, and semantic quality parameters such as CLIP between watermarked between watermarked images and non-watermarked images, which is beneficial for practical usage. When the watermark capacity increases to 64, the watermark component experiences convergence difficulties, leading to deviations of the latent variables from the standard Gaussian distribution. This issue is partly attributed that the specific structure of the watermark encoder and decoder poses difficulties in achieving the distribution of a 64-bit watermark. 

% \input{table_5}

% \section{3.Analysis on Sampling Method} 
% \label{sec3}
% Considering that untrustworthy parties might use different sampling patterns to circumvent the watermark embedding process, we conducted experiments with watermark embedding and unauthorized initial latent variable image generation using DDIM Scheduler \cite{song2020denoising}, DPMSolverMultistepScheduler \cite{lu2022dpm}, EulerAncestralDiscreteScheduler \cite{karras2022elucidating}, and HeunDiscreteScheduler \cite{karras2022elucidating}. Figure \ref{fig1} shows the images generated under different sampling methods for watermarked and non-watermarked latent variables. Under different sampling modes, Latent-VAE Skip-Binder remains effective. Random latent variables still fail to generate images correctly and images generated by watermarked initial latent variables remain the same. Some sampling modes such as EulerAncestralDiscreteScheduler do not support diffusion inversion, which can hinder watermark verification. We will continue to investigate this issue in future research.
% \begin{figure}[h]
% \centering
% \includegraphics[width=1\columnwidth]{3.png} % 
% \caption{Images generated from random latents and watermarked latents using different schedulers.}
% \label{fig1}
% \end{figure}

% \section{4.More Analysis on Image Processing Attack}
% \label{sec4}
% As shown in Figure \ref{fig1}, we consider image processing attack of different strength to evaluate the robustness of  the watermark including brightness, Gauss noise , Gauss blur , JPEG compression , image cropping, rotation, BM3D denoising algorithm, two VAE-based attacks and a diffusion based reconstructive attack. 
% The main experimental results are shown in Figure \ref{fig2}. From the figure, DistriMark demonstrates strong robustness against common attacks such as Brightness, Contrast, Resizing and Rescaling and JPEG Compression compared to other watermarking schemes for model distribution scenerios. It shows a clear advantage in dealing with more challenging attacks like VAE-based attacks and Diffusion-based attacks. DistriMark exhibits a certain level of robustness against Image Cropping, but its robustness is weaker for Image Cropping and Rescaling, as well as Image Rotation. 

% \begin{figure}[h]
% \centering
% \includegraphics[width=1\columnwidth]{v1.png} % 
% \caption{ Watermarked Image Subjected to Image Processing. 
%  (a) Original watermarked images. (b) Brightness adjustment of 2. (c) Gaussian noise with a standard deviation of 0.05. (d) Gaussian blur with a kernel size of 7×7. (e) JPEG compression with a quality factor of 50. (f) 20\% area crop. (g) 10\% random crop. (h) 20\% crop and scale. (i) Rotation by 45 degrees. 
%  (j) BM3D algorithm with a std of 0.1}
% \label{fig1}
% \end{figure}

% \begin{figure*}[h]
% \centering
% \includegraphics[width=2\columnwidth]{11.pdf} % 
% \caption{Evaluation on image processing.}
% \label{fig2}
% \end{figure*}

% \section{5.More Analysis on Watermark Embedding Efficiency}
% \label{sec5}
% For the 48-bit pretrained watermark encoder-decoder, it takes approximately 96 GPU hours to train. For fine-tuning the variational autoencoder for a specific model user, generating a single key only requires approximately 1 GPU hour on a single L40 GPU, which is practical for model distribution scenerios. Considering that the total training time for the diffusion model is about 150 to 1000 GPU days \cite{dhariwal2021diffusion}, the time spent on fine-tuning the model components is negligible. 
